# Supplementary material for: The pseudogap in hole-doped cuprates: possible insights from the Kondo effect
Source: arXiv:2108.02108 source file (2021-12-22)
Supplement: Supplementary file 1 [file Supp_Matv3.pdf]

# The pseudogap in hole-doped cuprates: possible insights from the Kondo effect. Supplemental Material

J. R. Cooper
*Cavendish Laboratory, Department of Physics, University of Cambridge, J.J. Thomson Avenue, CB3 0HE, United Kingdom*

(Dated: December 17, 2021)

Nine Figures are shown here, five are taken or adapted from other publications for convenience and four are for clarification of points made in the main paper.

## PROCEDURE USED TO DETERMINE $T_K$ AND CALCULATE THE ENTROPY IN THE SINGLE ION KONDO MODEL

The initial estimate of $T_K$ for Bi2212 from $\gamma(200)$ was 800 K. However specific heat calculations for the S = 1/2 Kondo model [1, 2] show that $\gamma(T = 0)$ is a factor of 1.19 larger than $\gamma(T/T_K = 0.25)$, i.e. $\gamma(200)$. So the initial estimate of $T_K$=800 K is reduced to 672 K. In order to compare theoretical $S_e(T)$ curves with the experimental data for representative samples of Bi2212 and YBCO we integrated the specific heat divided by $T$ calculated in [3]. This revealed a difficulty in that $\gamma(0)$ from [3] is exactly a factor 2 larger than the value in Eqn. 1. In principle this could be caused by the charge degrees of freedom [3], but we would expect such a contribution to become smaller as $|E_0|$ is increased and the Kondo limit is approached, see for example [4] Eqn. 5.20. In practice the calculated $\gamma(T/T_K)/\gamma(0)$ does not change as $-E_0/\Delta$ is varied from 4 to 2. Furthermore the $T$-dependence of $\gamma(T/T_K)/\gamma(0))$ agrees with the results of the Kondo model [1, 2] if the $T_K$ values in [3] are divided by a factor 2. This reduction then makes $\gamma(0)$ from [3] agree exactly with the value from [5] given in Eqn. 1.

So if our initial assumption that $\Delta = 1\ eV$ is correct then $T_K/\Delta$ = 800/(1.19x11600)= 0.058. Taking into account the decrease of a factor 2 in $T_K$, linear interpolation of the data in Table 1 of [3], gives $E_0/\Delta$ = -2.58. However Table 1 also shows that if $E_0/\Delta$ = -2.3 then the local level occupancy $n_0 = 0.81$. This corresponds to a localized moment of 0.81 $\mu_B$ and hence the susceptibility is reduced by a factor 0.69, giving a Wilson ratio of 1.31, rather close to the experimental value. Note that in insulating cupric salts, $Cu^{2+}$ is invariably an S=1/2 ion, and moreover often has similar $g$-factor anisotropy to that observed for YBCO crystals [7] and references therein, although admittedly it is not clear why magnetic defects in the CuO chains give an isotropic contribution [7] to the magnetic susceptibility. So therefore, contrary to initial expectations, we arrive at a value for $\Delta$ by requiring that $-E_0/\Delta \simeq 2.3$, hence $T_K/\Delta = 0.073$ (taking into account the factor of 2 explained above) and so $\Delta = 800/1.19/0.073/11600 = 0.79\ eV$. One minor effect of the above approach is that the half-widths of the resonances in Fig. 1(c) are now $\approx$ 1.5 to 2 x larger than $k_BT_K$

as shown by the horizontal arrows for $-E_0/\Delta = 2$ and 3.

**Calculations of $S_e(T)$ for representative Bi2212 and YBCO samples**

Figs. 7(SM) and 8(SM) show calculations for the present single ion model on the same scales as experimental data from Figs. 1(SM) and 2(SM), for critically-doped samples and samples with a pseudogap. It can be seen that subject to the caveats for YBCO mentioned in the figure caption there is good agreement between the experimental data and the model calculations.


[1] H.-U. Desgranges and K. D. Schotte, Specific heat of the Kondo model, Phys. Lett. **91A** 240 (1982).

[2] V. T. Rajan, Magnetic susceptibility and specific heat of the Coqblin-Schrieffer model, Phys. Rev. Lett. **51** 308-311 (1983).

[3] T. A. Costi, A. C. Hewson and V. Zlatić, Transport coefficients of the Anderson model via the numerical renormalization group, J. Phys.: Condens. Matter **6** 2519-2558 (1994).

[4] A. C. Hewson, "The Kondo problem to heavy fermions", Cambridge University Press, Cambridge, U.K. (1993).

[5] K. G. Wilson, Renormalization group- critical phenomena and Kondo problem, Rev. Mod. Phys. **47** 773-840 (1975).

[6] J. W. Loram, J. Luo, J. R. Cooper, W. Y. Liang and J. L. Tallon, Evidence on the pseudogap and condensate from the electronic specific heat, J. Phys. Chem. Solids **62**, 59-64 (2001).

[7] I. Kokanović and J. R. Cooper, Magnetic susceptibility of $YBa_2Cu_3O_{6+x}$ crystals: Unusual Curie behavior and small contributions from charge density waves, Phys. Rev. B **94** 075155-11 (2016).

[8] J. W. Loram, K. A. Mirza, J. R. Cooper and W. Y. Liang, Electronic specific heat of $YBa_2Cu_3O_{6+x}$ from 1.8 to 300 K, Phys. Rev. Lett. **71**, 1740-3 (1993).

[9] J. W. Loram, K. A. Mirza and J. R. Cooper, "IRC Research Review", pp 75-97, Ed. W. Y. Liang, University of Cambridge, Cambridge, U.K. (1998).

[10] S. Bermon, D. E. Paraskevopoulos and P. M. Tedrow, Ultra-high magnetic field study of the

Kondo-type zero-bias conductance peak in magnetically doped metal-insulator-metal tunnel junctions, Phys. Rev. B **17** 2110-2123 (1978).

[11] J. R. Cooper, H. Minami, V. W. Wittorff, D. Babić and J. W. Loram, Effect of the normal state gap on the thermoelectric power, irreversibility line and c-axis resistivity of $YBa_2Cu_3O_{7-\delta}$, Physica C **341** 855-858 (2000).

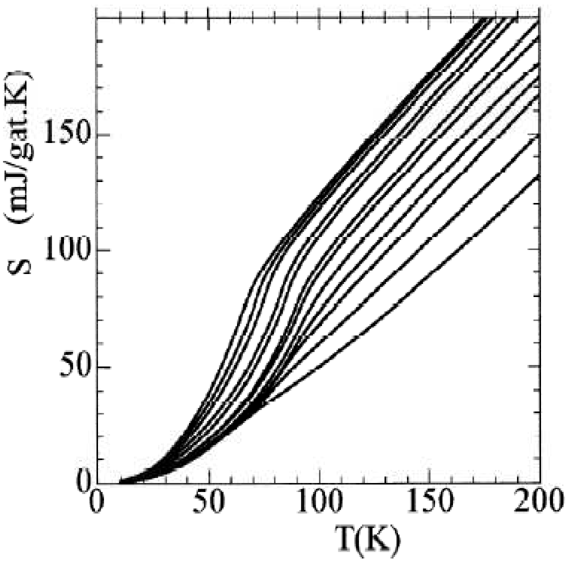


FIG. 1: Electronic entropy $S_e$ vs. $T$ for 20 % Pb doped and 15 % Y doped Bi2212 samples with $p$ varying from 0.095 (lowest value of $S$), to 0.22 (highest value of $S$), from Ref. [6].

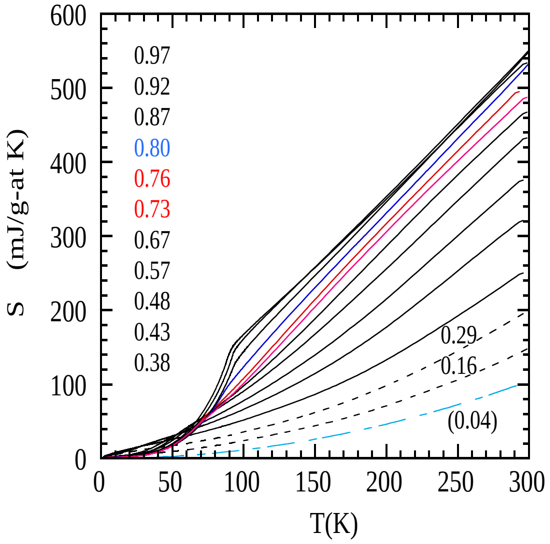


FIG. 2: Color online. Electronic entropy $S_e(x, T)$ of $YBa_2Cu_3O_{6+x}$ for the $x$-values shown, adapted from Refs. [8, 9].

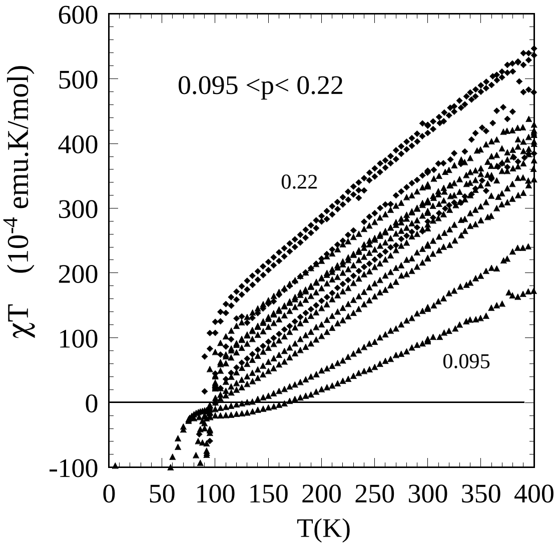


FIG. 3: The bulk susceptibility $\chi$, plotted as $\chi T$ vs. $T$ for 20 % Pb doped and 15 % Y doped Bi2212 samples with $p$ varying from 0.095 to 0.22, from Ref. [6].

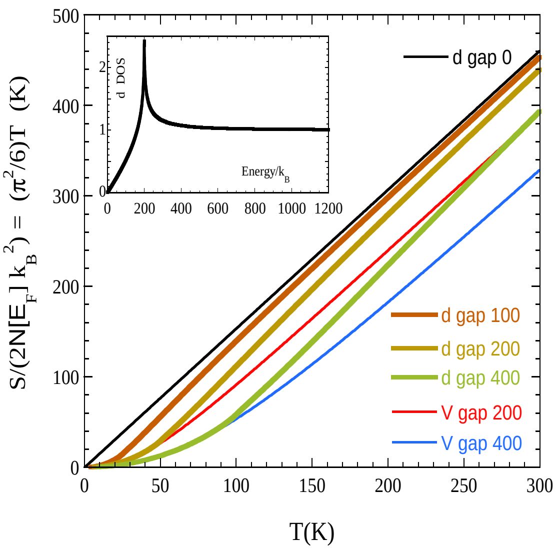


FIG. 4: Color online. Calculated electronic entropy, $S_e(T)$ for a states-conserving $d$ wave DOS (shown in the inset) with energy gap $\Delta/k_B$ = 100, 200 and 400 K and for the V-shaped states-non-conserving gap, shown in Fig.1(a) of the m/s, with $E_G/k_B$ = 200 and 400 K, both in a flat band, for the gap values shown. Note the tendency for the entropy to “come back” at higher $T$ for the states-conserving gap.

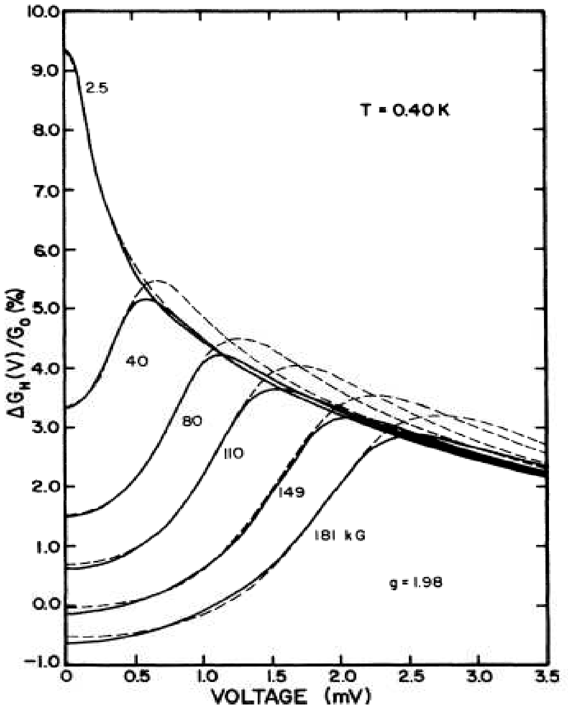


FIG. 5: Solid lines, experimental tunnelling conductance vs. bias voltage data for an $Al/Al_2O_3/Al$ junction doped with a fraction of a monolayer of Fe, Fig. 9 of Ref. [10] in various applied magnetic fields. Dashed lines show fits to theory available at that time. Note the states-non-conserving property of the experimental conductance, i.e. tunnelling DOS curves.

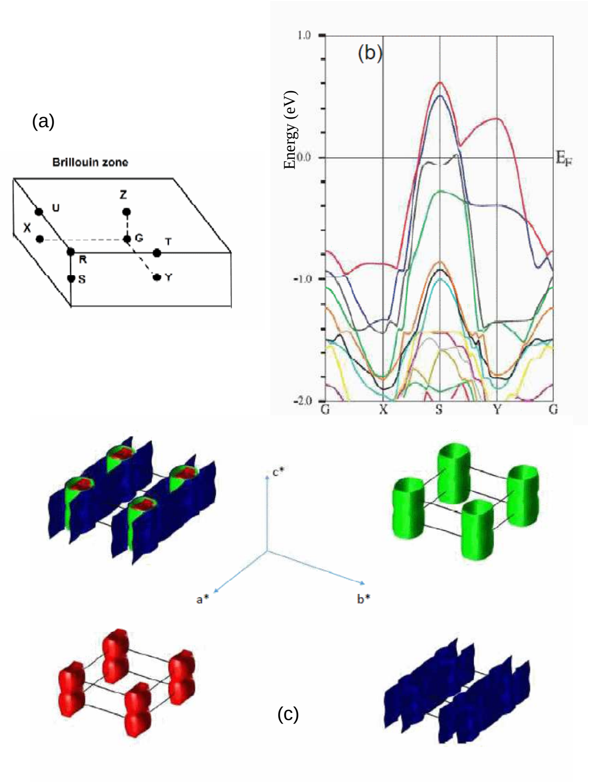


FIG. 6: Color online.(a) Brillouin zone showing symmetry points, (b) energy bands calculated for the hypothetical compound $YBa_2Zn_3O_7$, (c) calculated Fermi surface (FS) for the hypothetical compound $YBa_2Zn_3O_7$. Clockwise from top left: full FS, quasi-cylindrical sheet, open sheet and distorted cylindrical sheet. Directions in reciprocal space are shown.

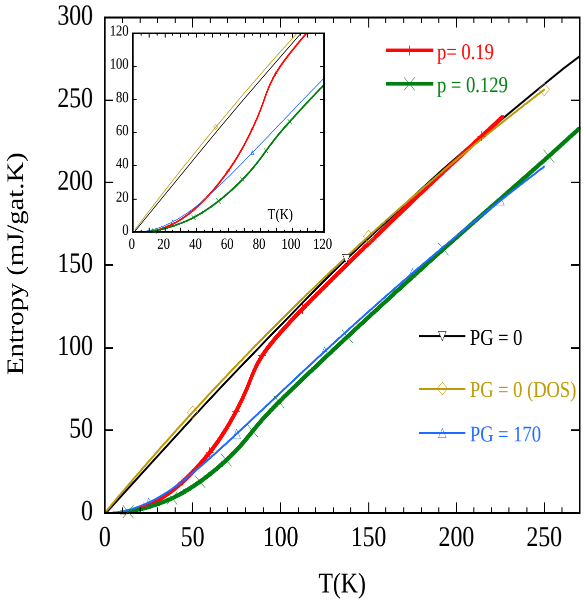


FIG. 7: Color online. Thicker lines with crosses, experimental data for Bi2212 from Fig. 1(SM). Thinner lines with various symbols, approximate fits to present model. Lines with $\bigtriangledown$, entropy obtained by integrating the calculated specific heat in Fig. 4 of Ref. [3] divided by $T$, for $E_0 = -2.5\Delta$ and $T_K = 672$ K for zero PG. On the scale used the curve for $E_0 = -2.3\Delta$ is the same as that for $E_0 = -2.5\Delta$. With $\diamond$, $S_e(T)$ generated by a suitable $E$-dependent DOS, which is then multiplied by a V-shaped function centered at $E_F$ to show the effect of the PG, lines with $\bigtriangleup$. The calculated and experimental $S_e(T)$ curves agree well up to 220 K.

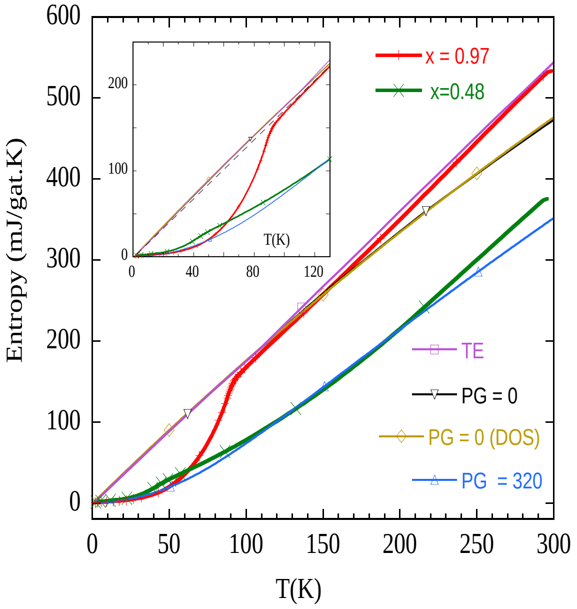


FIG. 8: Color online. Thicker lines with crosses, experimental data for $YBa_2Cu_3O_{6+x}$. Thinner lines with various symbols, approximate fits to present model. Lines with $\bigtriangledown$, entropy obtained by integrating the calculated specific heat in Fig. 4 of Ref. [3] divided by $T$, for $E_0 = -2.5\Delta$ and $T_K = 775$ K for zero PG. On the scale used the curve for $E_0 = -2.3\Delta$ is the same as that for $E_0 = -2.5\Delta$. With $\diamond$, $S_e(T)$ generated by a suitable $E$-dependent DOS, which is then multiplied by a V-shaped function centered at $E_F$ to show the effect of the PG, lines with $\triangle$. The differences between experimental and calculated $S_e(T)$ curves above 200 K could arise from a 15% decrease in $T_K$, between 100 and 300 K, from thermal expansion(TE), or because Cu atoms in the CuO chains are not equivalent to those in the $CuO_2$ planes. In the insert the dashed line shows that the calculated values of $S_e(T)$ with zero PG may well be slightly too high.

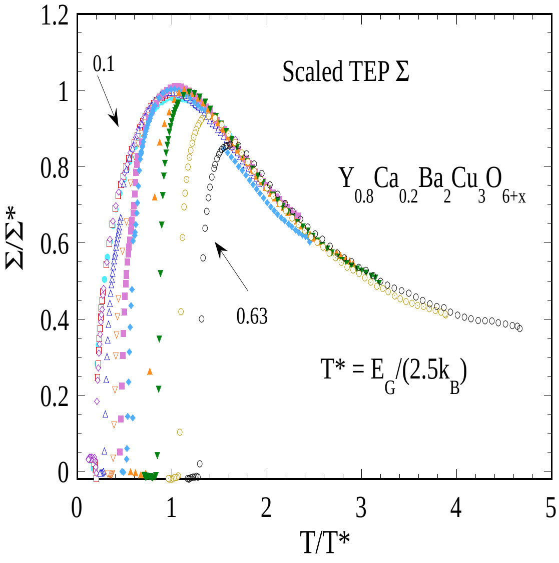


FIG. 9: Color online. Scaled thermoelectric power for $Y_{0.8}Ca_{0.2}Ba_2Cu_3O_{6+x}$, for $x$ between 0.1 and 0.63, adapted from [11].
